# Supplementary material for: The Next Evolution of Artificial Sense of Touch
Source: arXiv:2310.16641 source file (2023-12-21)
Supplement: Supplementary file 1 [file appendix.tex]

\section{Appendix}
Todo:
\begin{itemize}
    \item Include Haptic learning papers (Amartya) \sg{Done}
    \item Find papers on DNA materials \sg{Done}
\item Graph 1: Nanomaterials? Add a figure how TS with DNA could look in the future, electronics chemical, 6G, molecular factory finds materials assembles and tests them (Sonja) \sg{Done}
\item quantum computing \sg{Done}
\item Graph 2: not colored more dotted lines, human emphasized, captions below \sg{Done}
\item do estimates for human and change line of argument (we need nanomaterials because adding current state is not possible), add NaN, \sg{Done}
\item We need to increase TS technology (give requirements) estimates on how NM \sg{Done}
\item vectorize graphs \sg{Done}
\item double check maximum values for soA \sg{To Do}
\end{itemize}
\mycomment{
\begin{figure}
\centering
\includegraphics[width=\textwidth]{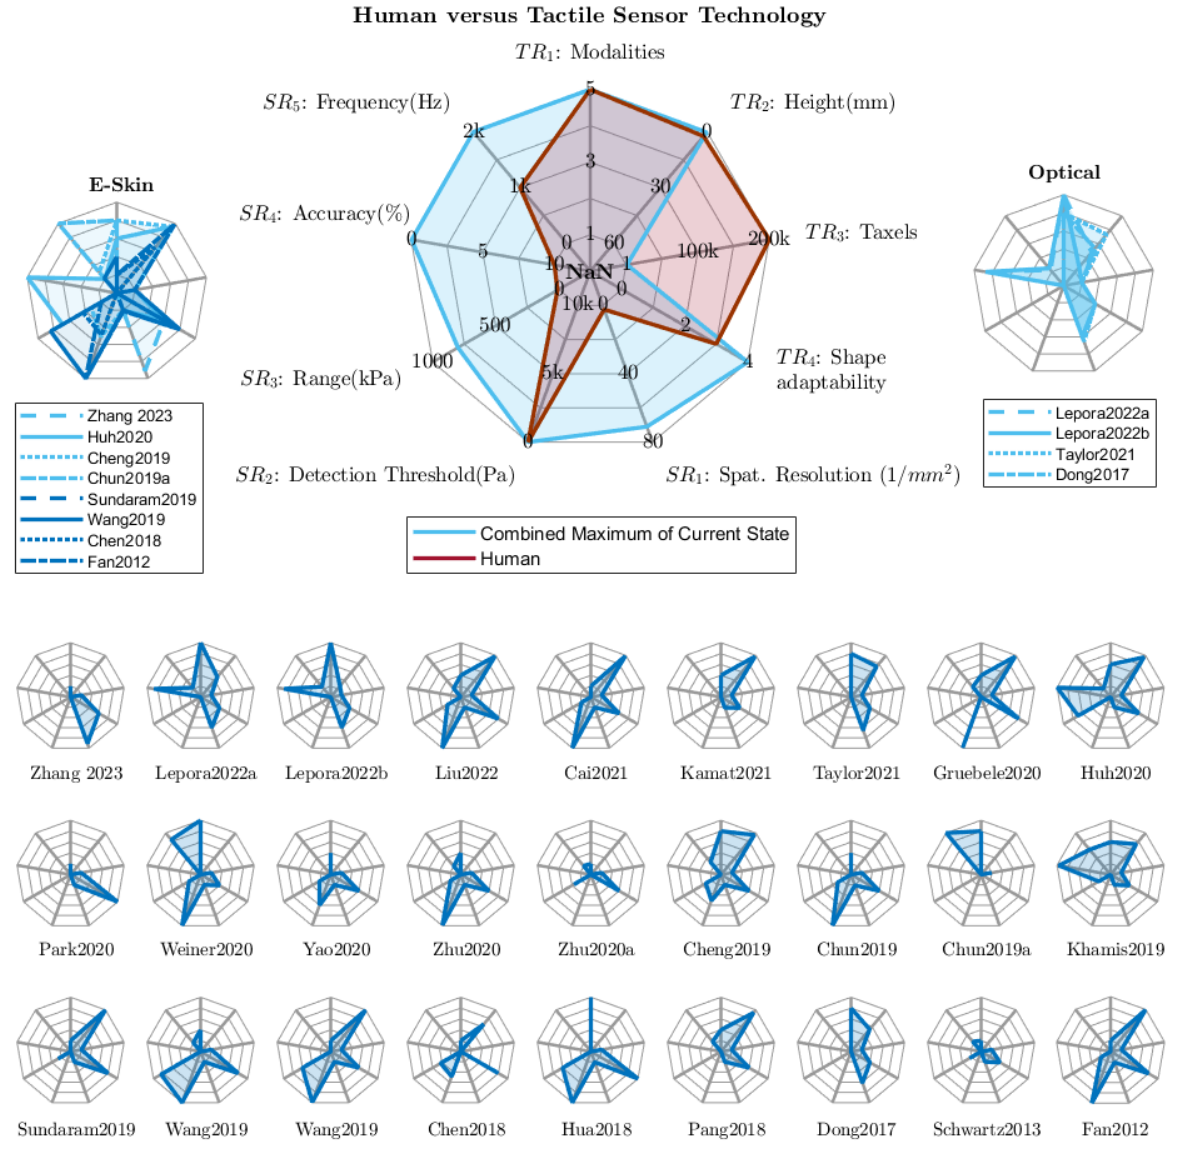}
\caption{Quantitative and qualitative comparison of characteristics for tactile sensing prototypes in comparison to human tactile sensing. We evaluated technical ($TR_1-TR_4$) and sensing requirements ($SR_1-SR_5$): $TR_1$: Amount of modalities (1-5), $TR_2$: Heigth (mm), $TR_3$: Amount of taxels, $TR_4$: Conformability (rigid/compliant (1), bendable (2), stretchable (3), highly stretchable $>200$~$\%$ (4)), $SR_1$: Spatial resolution (taxel/mm$^2$), $SR_2$: Detection threshold for pressure (kPa), $SR_3$:  Pressure Range (kPa), $SR_4$: Accuracy of force estimation (in $\%$ with regard to range), $SR_5$: sensor frequency (Hz). Estimations for human skin properties from \cite{Brandes2019,Oltulu2018,Corniani2020,Dargahi2004, Annaidh2012,Zhang2023,Pyo2021,Saal2016}, \cite{Knibestoel1980}\sg{find newer reference for accuracy?}.}
\label{fig:sp}
\end{figure}

\begin{figure}
\centering
\includegraphics[width=\textwidth]{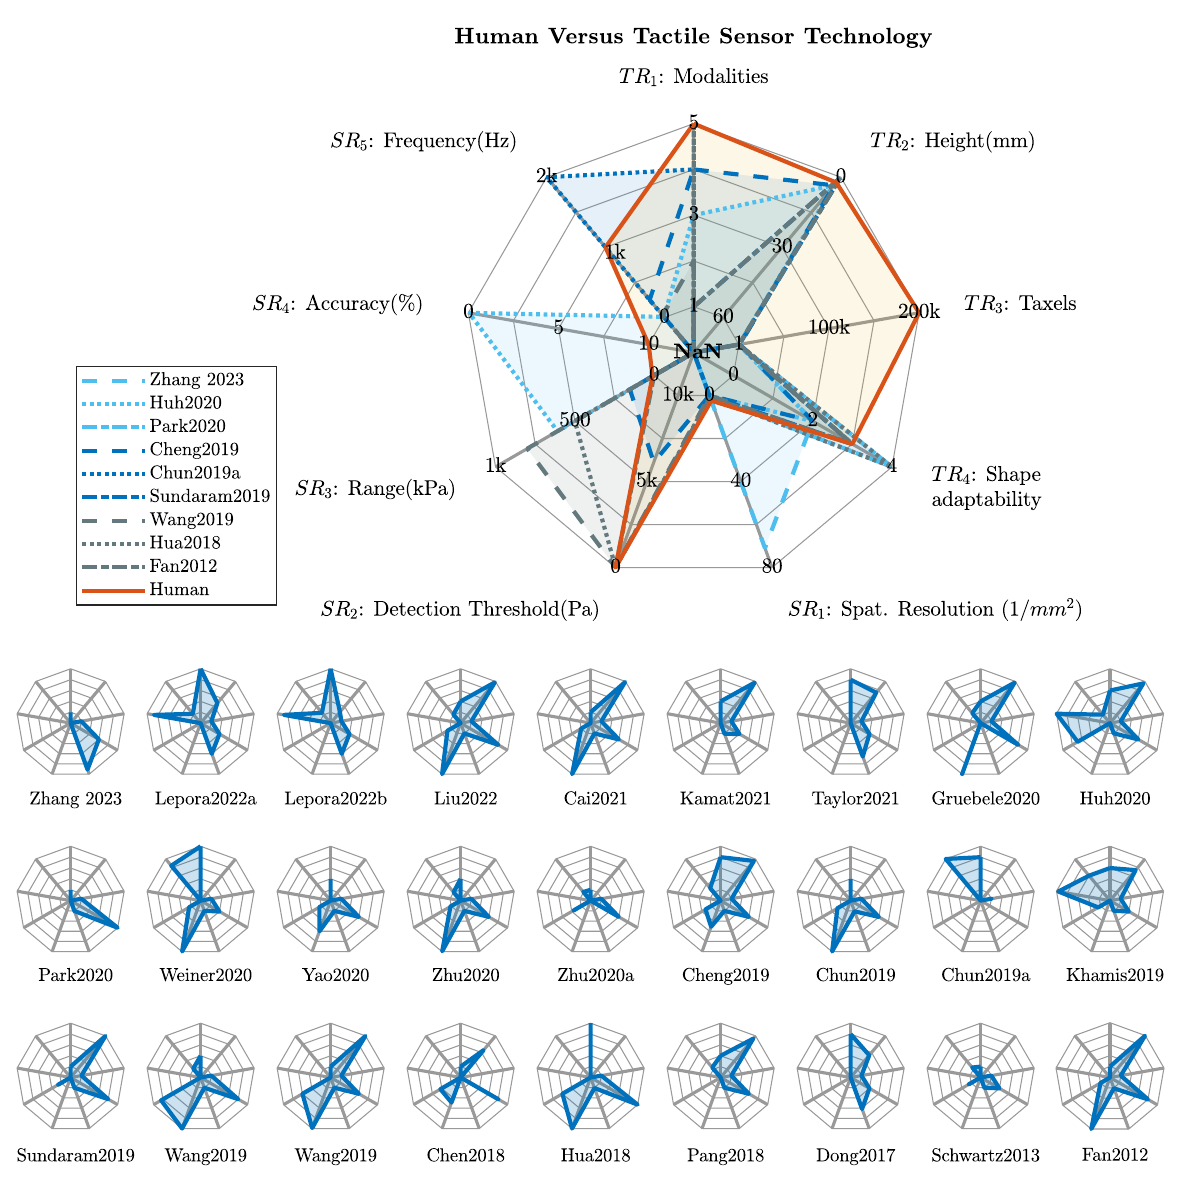}
\caption{\sg{Alternative.} Quantitative and qualitative comparison of characteristics for tactile sensing prototypes in comparison to human tactile sensing. We evaluated technical ($TR_1-TR_4$) and sensing requirements ($SR_1-SR_5$): $TR_1$: Amount of modalities (1-5), $TR_2$: Heigth (mm), $TR_3$: Amount of taxels, $TR_4$: Conformability (rigid/compliant (1), bendable (2), stretchable (3), highly stretchable $>200$~$\%$ (4)), $SR_1$: Spatial resolution (taxel/mm$^2$), $SR_2$: Detection threshold for pressure (kPa), $SR_3$:  Pressure Range (kPa), $SR_4$: Accuracy of force estimation (in $\%$ with regard to range), $SR_5$: sensor frequency (Hz). Estimations for human skin properties from \cite{Brandes2019,Oltulu2018,Corniani2020,Dargahi2004, Annaidh2012,Zhang2023,Pyo2021,Saal2016}, \cite{Knibestoel1980} \sg{find newer reference for accuracy?}.}
\label{fig:sp}
\end{figure}}

\mycomment{
- Robots with embodies neuromorphic intelligence : \cite{Bartolozzi2022}, for reflexes , sensors \cite{Sun2022, Liu2022}, electronics \cite{Ham2021}, 
- multisensory fusion for texture recognition \cite{Rostamian2022}
}

\mycomment{
\begin{figure}
\centering
\includegraphics[width=0.95\textwidth]{figures/overview2.png}
\caption{Alternative with Garmi. \ag{Ensure you have permission to use these figures.}}
\label{fig:TS_a}
\end{figure}}

\mycomment{
\begin{figure}
\centering
\begin{subfigure}{0.7\textwidth}
\includegraphics[width=1\textwidth]{figures/sp7.png}
\end{subfigure}
\hfill
\begin{subfigure}{0.7\textwidth}
\includegraphics[width=\textwidth]{figures/sp6.png}
\end{subfigure}
\caption{Quantitative and qualitative comparison of sensor characteristics for camera-based and e-Skin approaches. Evaluated characteristics: Amount of modalities (1-5), detection threshold for pressure (N), pressure Range (kPa), implemented taxel scalability (amount of taxels), spatial resolution (taxel/mm$^2$), conformability (rigid/compliant (1), bendable (2), stretchable (3), highly stretchable $>200$~$\%$ (4)), accuracy (in $\% $ with regard to range), detected frequency range (Hz).}
\label{fig:sp5}
\end{figure}
}
\mycomment{
\paragraph{Availability}
Only few multi-modal, compliant sensory systems have reached the commercial market. 
\cite{Syntouch2021} offers the BioTac, a multi-modal sensorized fingertip for robotic hands and a low-cost version called NumaTac with lower complexity. Furthermore, \cite{Contactile2021} provides an optical solution that uses photodiodes to measure contact points (3x3 arrays), 3D forces and vibration. Robot Collision detection systems with integrated damping are offered by \cite{Airskin}, although they are lacking sufficient spatial resolution and shear-force detection.
}
\mycomment{\sg{Open question: why do we want to achieve human-like tactile sensing? Actually the requirements for tactile sensing are not really clear. Do we really need human-like data density?}
\sh{Well ideally, we would like to go even beyond. Any technical sensor has so far always turned out to be better than any biological counterpart in the past (torque sensing, position sensing, gyros, acceleration, ...). I would rather say it is reasonable to at least target the human level.}}

\mycomment{In the long term, it might be promising to consider quantum computing for instantaneous and safe data transmission \cite{Fettweis2022}.}

\mycomment{
Moreover, new computational design and modeling algorithms are required to achieve and manage the required data density. }
\mycomment{
    \item Miniaturization (well, in fact, the big change is instead of top down engineering way of skin design and production, let us leverage nano-level properties, their constructive capabilities, ..., 
    \item Printability
    \item Stretchability
\item Growing materials could have huge potential}

\mycomment{
\begin{figure}
\centering
\includegraphics[width=0.8\textwidth]{figures/sp5.png}
\caption{}
\label{fig:persp}
\end{figure}}

\mycomment{What is the Gap in tactile sensing technology?
\begin{itemize}
    \item Long-term stability 
    \item Power consumption
    \item Amount Data/ Processing
    \item Durability/ environmental stability
    \item Large area, high density, thin, soft and multi-modal implementation
    \item Combination of requirements
    \item Level of integration with multiple modalities
    \item Fast data lines?--> quantum computing?
\end{itemize}
How can Non-materials/Microstructures close that gap?
\begin{itemize}
    \item Higher sensitivity of functional materials 
    \item Multi-modal structures/ principles
    \item Miniaturization
    \item Printability
    \item Stretchability
    \item Decreased toxicity
    \item Biomimetic characteristics:
    Self-healing, 
Energy harvesting (TENGs),
Self learning,
Integrated processing,
Wireless communication,
Neural spikes for smart processing
\end{itemize}}

\mycomment{Cytotoxicity refers to a substance's ability to harm cells.}

\mycomment{The development of high-performance biosensing capabilities within wearable electronics is a pivotal focus area for achieving truly dexterous manipulation capabilities in robots. This encompasses advancing implantable sensors, electronic skin (e-skins), and interactive human-machine electronics. Inspired by the somatosensory system found in biological skin, e-skins have incorporated a range of physical transduction mechanisms \cite{abraira2013sensory, delmas2011molecular}. These mechanisms include capacitance \cite{zhao2021shape}, piezoresistivity \cite{choong2014highly}, and piezoelectricity \cite{wu2022prospects}. Additionally, self-healing and self-powered electronic systems have recently been introduced. These innovations are highly sought after to create advanced multifunctional e-skins with exceptional sensitivity in the next generation.
\ag{Hydrogels have the potential to serve as wearable sensors capable of accurately detecting a wide range of human movements and physiological signals \cite{zhang2022flexible}. These signals include joint motions, facial expressions, voice patterns, and breathing. A strategy inspired by DNA has opened the door to the systematic design of hydrogels with mechanical properties similar to human skin. This innovation holds great promise for applications in intelligent wearable devices, human-machine interfaces, and soft robotics \cite {zhang2021dna}}}
